# Supplementary material for: Active Representation Learning for General Task Space with Applications in Robotics
Source: arXiv:2306.08942 source file (2023-06-15)
Supplement: Supplementary file 1 [file appendix.tex]

% \section{Results and analysis for Target-aware}

% Results and analysis for Target-aware
\section{Result and analysis for target-aware}
\label{sec: target-aware (appendix)}
\input{appendix-generalization1}
\input{appendix-sampleComplexity1}
\input{appendix-resultComparison}

% Results and analysis for Target-agnostic
\input{appendix-targetAgnostic}

% More experiments
\input{appendix-experiment}
